# Supplementary material for: Amortized Monte Carlo Integration
Source: arXiv:1907.08082 source file (2019-07-18)
Supplement: Supplementary file 2 [file appendix-positivisation.tex]

\section{Positivisation}
\label{sec:positivisation}

Positivisation uses multiple importance samplers to allows one to formulate a zero variance estimator when $f(x)$ takes both positive and negative signs, and is not upper or lower bounded.
Following \citet{Owen2013}, we use a standard decomposition of $f(x)$ into positive and negative parts.
Define
$f_+(x) = \max(f(x), 0)$, and
$f_-(x) = \max(-f(x), 0)$.
Then $f(x) = f_+(x) -f_-(x)$.

Now let $q_+(x)$ be a density function which is positive whenever $p(x)f_+(x) > 0$ and
let $q_-(x)$ be a density function which is positive whenever $p(x)f_-(x) > 0$. 
We take $n_\pm$ samples $x^+_a$, $x^-_b$ from $q_\pm(x)$ respectively.
The estimator for $\E_{p(x)}\!\left[f(x)\right]$ is
\begin{align}
\E_{p(x)}\!\left[f(x)\right]
=
\frac{1}{n_+} \sum_{a}^{n_+} \frac{f_+(x^+_a)p(x^+_a)}{q_+(x^+_a)}
-
\frac{1}{n_-} \sum_{b}^{n_-} \frac{f_-(x^-_b)p(x^-_b)}{q_-(x^-_b)}
\end{align}
The optimal sampling proposals are $q_\pm(x) \propto p(x)f_\pm(x)$, respectively.
If optimal sampling proposals are used we get zero variance for sample budget $n_+ = n_- = 1$, i.e. $n=2$.

In the AMCI setting positivisation affects the estimator of 
$\E_{p(x|y)}[f(x)]$ from \eqref{eq:estimator-combination}.
It also implies that we need to learn three instead of two proposal distributions, which we will denote as $q_{1+}(x|y), q_{1-}(x|y)$ and $q_{2}(x|y)$.
Instead of drawing $N$ samples from $q_1(x|y; \eta)$, we now draw $n_+, n_-$ samples $x^+_a, x^-_b$ from $q_1+, q_1-$, respectively, such that $n_+ + n_- = N$. 
We also draw $M$ samples $x^*_m$ from $q_2$.
The new form of the estimator is
\begin{align} 
\E_{p(x)}\!\left[f(x)p(y|x)\right] 
= 
&\,\,
\alpha \left( 
\frac{1}{n_+} \sum_a^{n_+} \!\frac{f_+(x^+_a) p(x^+_a, y) }{q_{1+}(x^+_a|y)} 
-
\frac{1}{n_-} \sum_b^{n_-} \!\frac{f_-(x^-_b) p(x^-_b, y) }{q_{1-}(x^-_b|y)} 
\right)
\nonumber \\
&+ \frac{1-\alpha}{M} \sum_m^M \!\frac{f(x_m^*) p(x_m^*, y)}{q_2(x_m^*|y)}\\
\E_{p(x)}\!\left[p(y|x)\right] 
= 
&\,\,
\beta \left( 
\frac{1}{n_+} \sum_a^{n_+} \!\frac{p(x^+_a, y) }{q_{1+}(x^+_a|y)} 
+
\frac{1}{n_-} \sum_b^{n_-} \!\frac{p(x^-_b, y) }{q_{1-}(x^-_b|y)} 
\right)
\nonumber \\
&+ \frac{1-\beta}{M} \sum_m^M \!\frac{p(x_m^*, y)}{q_2(x_m^*|y)}\\
\E_{p(x|y)}[f(x)]
=& \,\,
\frac{\E_{p(x)} \! \left[ f(x)p(y|x) \right] }{\E_{p(x)}\! \left[ p(y|x) \right]}
\end{align}
